# Supplementary material for: A Momentum-Resolved X-ray Thomson Scattering Benchmark of Electronic-Response Models in Warm Dense Aluminium
Source: arXiv:2509.10107 source file (2026-05-06)
Supplement: Supplementary file 1 [file supp_main.tex]

\input{preamble.tex}
\sisetup{
  range-phrase   = --,
  range-units    = single,
  uncertainty-mode = separate
}

\usepackage{comment}

\begin{document}

\title{Supplemental Material for ``A Momentum-Resolved X-ray Thomson Scattering Benchmark of Electronic-Response Models in Warm Dense Aluminium''}

\author{Dmitrii S. Bespalov}
\email{dmitrii.bespalov@xfel.eu}
\affiliation{European XFEL, Holzkoppel 4, 22869 Schenefeld, Germany}
\affiliation{Institute of Physics, University of Rostock, Albert-Einstein-Straße 23-24, 18059 Rostock, Germany}

\author{Ulf Zastrau}
\affiliation{European XFEL, Holzkoppel 4, 22869 Schenefeld, Germany}

\author{Zhandos A. Moldabekov}
\affiliation{Institute of Radiation Physics, Helmholtz-Zentrum Dresden-Rossendorf (HZDR), D-01328 Dresden, Germany}
\affiliation{Helmholtz-Zentrum Dresden-Rossendorf (HZDR), D-01328 Dresden, Germany}

\author{Thomas Gawne}
\affiliation{Center for Advanced Systems Understanding (CASUS), D-02826 G\"orlitz, Germany}
\affiliation{Helmholtz-Zentrum Dresden-Rossendorf (HZDR), D-01328 Dresden, Germany}

\author{Tobias Dornheim}
\affiliation{Institute of Radiation Physics, Helmholtz-Zentrum Dresden-Rossendorf (HZDR), D-01328 Dresden, Germany}
\affiliation{Center for Advanced Systems Understanding (CASUS), D-02826 G\"orlitz, Germany}
\affiliation{Helmholtz-Zentrum Dresden-Rossendorf (HZDR), D-01328 Dresden, Germany}

\author{Moyassar Meshhal}
\affiliation{Institute of Physics, University of Rostock, Albert-Einstein-Straße 23-24, 18059 Rostock, Germany}

\author{Alexis Amouretti}
\affiliation{Osaka University, Graduate School of Engineering Science, 1-3 Machikaneyama, Toyonaka, Osaka 560-8531, Japan}
\affiliation{European Synchrotron Radiation Facility (ESRF), 71 Avenue des Martyrs, CS 40220, 38043 Grenoble Cedex 9, France}

\author{Michal Andrzejewski}
\affiliation{European XFEL, Holzkoppel 4, 22869 Schenefeld, Germany}

\author{Karen Appel}
\affiliation{European XFEL, Holzkoppel 4, 22869 Schenefeld, Germany}

\author{Carsten Baehtz}
\affiliation{Helmholtz-Zentrum Dresden-Rossendorf (HZDR), D-01328 Dresden, Germany}

\author{Erik Brambrink}
\affiliation{European XFEL, Holzkoppel 4, 22869 Schenefeld, Germany}

\author{Khachiwan Buakor}
\affiliation{European XFEL, Holzkoppel 4, 22869 Schenefeld, Germany}

\author{Carolina Camarda}
\affiliation{European XFEL, Holzkoppel 4, 22869 Schenefeld, Germany}

\author{David Chin}
\affiliation{University of Rochester, Laboratory for Laser Energetics (LLE), 250 East River Road, Rochester, NY 14623, USA}

\author{Gilbert Collins}
\affiliation{University of Rochester, Laboratory for Laser Energetics (LLE), 250 East River Road, Rochester, NY 14623, USA}
\affiliation{University of Oxford, Department of Physics, Clarendon Laboratory, Parks Road, Oxford OX1 3PU, United Kingdom}

\author{C\'eline Cr\'episson}
\affiliation{University of Oxford, Department of Physics, Clarendon Laboratory, Parks Road, Oxford OX1 3PU, United Kingdom}

\author{Adrien Descamps}
\affiliation{Queen's University Belfast, School of Maths and Physics, University Road, Belfast BT7 1NN, United Kingdom}

\author{Jon Eggert}
\affiliation{Lawrence Livermore National Laboratory (LLNL), Physical \& Life Sciences, 7000 East Avenue, Livermore, CA 94550, USA}

\author{Luke Fletcher}
\affiliation{Stanford University and SLAC National Accelerator Laboratory, SIMES, Stanford, CA 94305, USA}

\author{Alessandro Forte}
\affiliation{University of Oxford, Department of Physics, Clarendon Laboratory, Parks Road, Oxford OX1 3PU, United Kingdom}

\author{Gianluca Gregori}
\affiliation{University of Oxford, Department of Physics, Clarendon Laboratory, Parks Road, Oxford OX1 3PU, United Kingdom}

\author{Marion Harmand}
\affiliation{CNRS -- DSI Meudon, Laboratoire PIMM (UMR 8006), ENSAM/CNAM, 155 Bd de l'H\^opital, 75013 Paris, France}

\author{Oliver S. Humphries}
\affiliation{European XFEL, Holzkoppel 4, 22869 Schenefeld, Germany}

\author{Hauke H\"oppner}
\affiliation{Helmholtz-Zentrum Dresden-Rossendorf (HZDR), D-01328 Dresden, Germany}

\author{Jonas Kuhlke}
\affiliation{Helmholtz-Zentrum Dresden-Rossendorf (HZDR), D-01328 Dresden, Germany}

\author{William Lynn}
\affiliation{Queen's University Belfast, School of Maths and Physics, University Road, Belfast BT7 1NN, United Kingdom}

\author{Julian L\"utgert}
\affiliation{Institute of Physics, University of Rostock, Albert-Einstein-Straße 23-24, 18059 Rostock, Germany}

\author{Masruri Masruri}
\affiliation{Helmholtz-Zentrum Dresden-Rossendorf (HZDR), D-01328 Dresden, Germany}

\author{Emma M. McBride}
\affiliation{Queen's University Belfast, School of Maths and Physics, University Road, Belfast BT7 1NN, United Kingdom}

\author{Ryan Stewart McWilliams}
\affiliation{The University of Edinburgh, School of Physics and Astronomy, JCMB, Peter Guthrie Tait Road, Edinburgh EH9 3FD, United Kingdom}

\author{Alan Augusto Sanjuan Mora}
\affiliation{Institute of Physics, University of Rostock, Albert-Einstein-Straße 23-24, 18059 Rostock, Germany}

\author{Jean-Paul Naedler}
\affiliation{Institute of Physics, University of Rostock, Albert-Einstein-Straße 23-24, 18059 Rostock, Germany}

\author{Paul Neumayer}
\affiliation{GSI Helmholtzzentrum f\"ur Schwerionenforschung, Postfach 11 05 52, 64278 Darmstadt, Germany}

\author{Charlotte Palmer}
\affiliation{Queen's University Belfast, School of Maths and Physics, University Road, Belfast BT7 1NN, United Kingdom}

\author{Alexander Pelka}
\affiliation{Helmholtz-Zentrum Dresden-Rossendorf (HZDR), D-01328 Dresden, Germany}

\author{Lea Pennacchioni}
\affiliation{Universit\"at Potsdam, Institut f\"ur Geowissenschaften, Karl-Liebknecht-Str. 24-25, 14476 Potsdam-Golm, Germany}

\author{Calum Prestwood}
\affiliation{European XFEL, Holzkoppel 4, 22869 Schenefeld, Germany}
\affiliation{Queen's University Belfast, School of Maths and Physics, University Road, Belfast BT7 1NN, United Kingdom}

\author{Natalia A. Pukhareva}
\affiliation{Institute for Materials, Ruhr-Universit\"at Bochum, Universit\"atsstr. 150, 44801 Bochum, Germany}

\author{Chongbing Qu}
\affiliation{Institute of Physics, University of Rostock, Albert-Einstein-Straße 23-24, 18059 Rostock, Germany}

\author{Divyanshu Ranjan}
\affiliation{DESY, Photon Science, Notkestrasse 85, 22607 Hamburg, Germany}
\affiliation{Institute of Physics, University of Rostock, Albert-Einstein-Straße 23-24, 18059 Rostock, Germany}

\author{Ronald Redmer}
\affiliation{Institute of Physics, University of Rostock, Albert-Einstein-Straße 23-24, 18059 Rostock, Germany}

\author{Michael R\"oper}
\affiliation{DESY, Photon Science, Notkestrasse 85, 22607 Hamburg, Germany}

\author{Christoph Sahle}
\affiliation{European Synchrotron Radiation Facility (ESRF), 71 Avenue des Martyrs, CS 40220, 38043 Grenoble Cedex 9, France}

\author{Samuel Schumacher}
\affiliation{Institute of Physics, University of Rostock, Albert-Einstein-Straße 23-24, 18059 Rostock, Germany}

\author{Jan-Patrick Schwinkendorf}
\affiliation{Helmholtz-Zentrum Dresden-Rossendorf (HZDR), D-01328 Dresden, Germany}

\author{Melanie J. Sieber}
\affiliation{Universit\"at Potsdam, Institut f\"ur Geowissenschaften, Karl-Liebknecht-Str. 24-25, 14476 Potsdam-Golm, Germany}

\author{Madison Singleton}
\affiliation{SLAC National Accelerator Laboratory, LCLS, 2575 Sand Hill Road, MS103, Menlo Park, CA 94025, USA}

\author{Ethan Smith}
\affiliation{University of Rochester, Laboratory for Laser Energetics (LLE), 250 East River Road, Rochester, NY 14623, USA}

\author{Christian Sternemann}
\affiliation{DELTA / Fakult\"at Physik, Technische Universit\"at Dortmund, Maria-Goeppert-Mayer-Str. 2, 44227 Dortmund, Germany}

\author{Thomas Stevens}
\affiliation{University of Oxford, Department of Physics, Clarendon Laboratory, Parks Road, Oxford OX1 3PU, United Kingdom}

\author{Michael Stevenson}
\affiliation{Institute of Physics, University of Rostock, Albert-Einstein-Straße 23-24, 18059 Rostock, Germany}

\author{Cornelius Strohm}
\affiliation{DESY, Photon Science, Notkestrasse 85, 22607 Hamburg, Germany}

\author{Minxue Tang}
\affiliation{DESY, Photon Science, Notkestrasse 85, 22607 Hamburg, Germany}

\author{Monika Toncian}
\affiliation{Helmholtz-Zentrum Dresden-Rossendorf (HZDR), D-01328 Dresden, Germany}

\author{Toma Toncian}
\affiliation{Helmholtz-Zentrum Dresden-Rossendorf (HZDR), D-01328 Dresden, Germany}

\author{Thomas Tschentscher}
\affiliation{European XFEL, Holzkoppel 4, 22869 Schenefeld, Germany}

\author{Sam M. Vinko}
\affiliation{University of Oxford, Department of Physics, Clarendon Laboratory, Parks Road, Oxford OX1 3PU, United Kingdom}

\author{Justin S. Wark}
\affiliation{University of Oxford, Department of Physics, Clarendon Laboratory, Parks Road, Oxford OX1 3PU, United Kingdom}

\author{Max Wilke}
\affiliation{Universit\"at Potsdam, Institut f\"ur Geowissenschaften, Karl-Liebknecht-Str. 24-25, 14476 Potsdam-Golm, Germany}

\author{Dominik Kraus}
\affiliation{Institute of Physics, University of Rostock, Albert-Einstein-Straße 23-24, 18059 Rostock, Germany}

\author{Thomas R. Preston}
\email{thomas.preston@xfel.eu}
\affiliation{European XFEL, Holzkoppel 4, 22869 Schenefeld, Germany}

\date{\today}

\maketitle
\onecolumngrid

\beginsupplement

\SMsection{Hydrodynamics, timing, and density averaging}{sec:S1}

\textbf{Hydrodynamic simulations and timing calibration.}
Target compression was modelled with the 1D Lagrangian radiation-hydrodynamics code HELIOS-CR~\cite{macfarlane2006helios}, using the full Kapton/epoxy/Al target stack and the experimental laser parameters. The incident drive was represented as an 8~ns flat-top pulse at 515~nm, focused to a $\sim250~\mu$m super-Gaussian spot at $22.5^\circ$ incidence, with a nominal pulse energy of $\sim26$~J. The absorbed drive energy was calibrated by matching the HELIOS-CR breakout time to the optical breakout measured by VISAR, yielding an effective absorbed energy of 19~J ($\simeq75\%$ of the nominal 26~J after optical losses and ablator reflectivity). Representative VISAR data and the 1D hydrodynamic profiles used in the main validation package are shown in the End Matter (the VISAR and hydrodynamic-profile figures). The XFEL probe time was fixed at $t_\mathrm{pp}=6.3$~ns, strictly before breakout for all angles, and the VISAR-measured breakout remained stable at $t_\mathrm{b}=6.5\pm0.1$~ns across the shot set.

HELIOS-CR simulations are inherently one-dimensional and do not resolve lateral inhomogeneities or edge effects near the focal spot. However, given the $\sim250~\mu$m DiPOLE drive spot, the $\sim35~\mu$m XFEL probe size, and the $50~\mu$m Al thickness, transverse gradients are expected to be negligible within the central region probed by XRTS and XRD, so that 1D profiles provide an adequate description of the local drive conditions.

\textbf{State at probe time and density window.}
Profiles extracted at $t_\mathrm{pp}=6.3$~ns show a stable compressed Al region with density spanning $3.75$--$4.5~\mathrm{g\,cm^{-3}}$ and an approximately uniform temperature of $T \approx 0.6~\si{\electronvolt}$. Over the central $\sim30~\mu$m plateau the density varies by about $20\%$, while $T$ is flat to within about $2\%$ (Fig.~\ref{fig:hydro_2d} and the End Matter hydrodynamic-profile figure). This density range defines the window used for all theory-data comparisons and for the density averaging applied to computed dynamic structure factors,
\begin{equation}
  S_{\mathrm{avg}}(k,\omega)
  = \frac{1}{N}\sum_{i=1}^{N}
    S\!\left(k,\omega;\rho_i,T\right),
  \qquad
  N=4,
\end{equation}
where the $\rho_i$ are equally spaced over the experimentally constrained density interval at fixed $T \approx 0.6~\si{\electronvolt}$. Independent XRD analysis of the driven shots yields an ionic structure factor consistent with DFT-MD predictions in the same density window (the main-text XRTS/XRD comparison figure and Sec.~S8), supporting the HELIOS-CR state assignment.

\begin{figure*}[ht]
\centering

\begin{overpic}[width=0.49\linewidth,trim=190 140 120 120,clip]{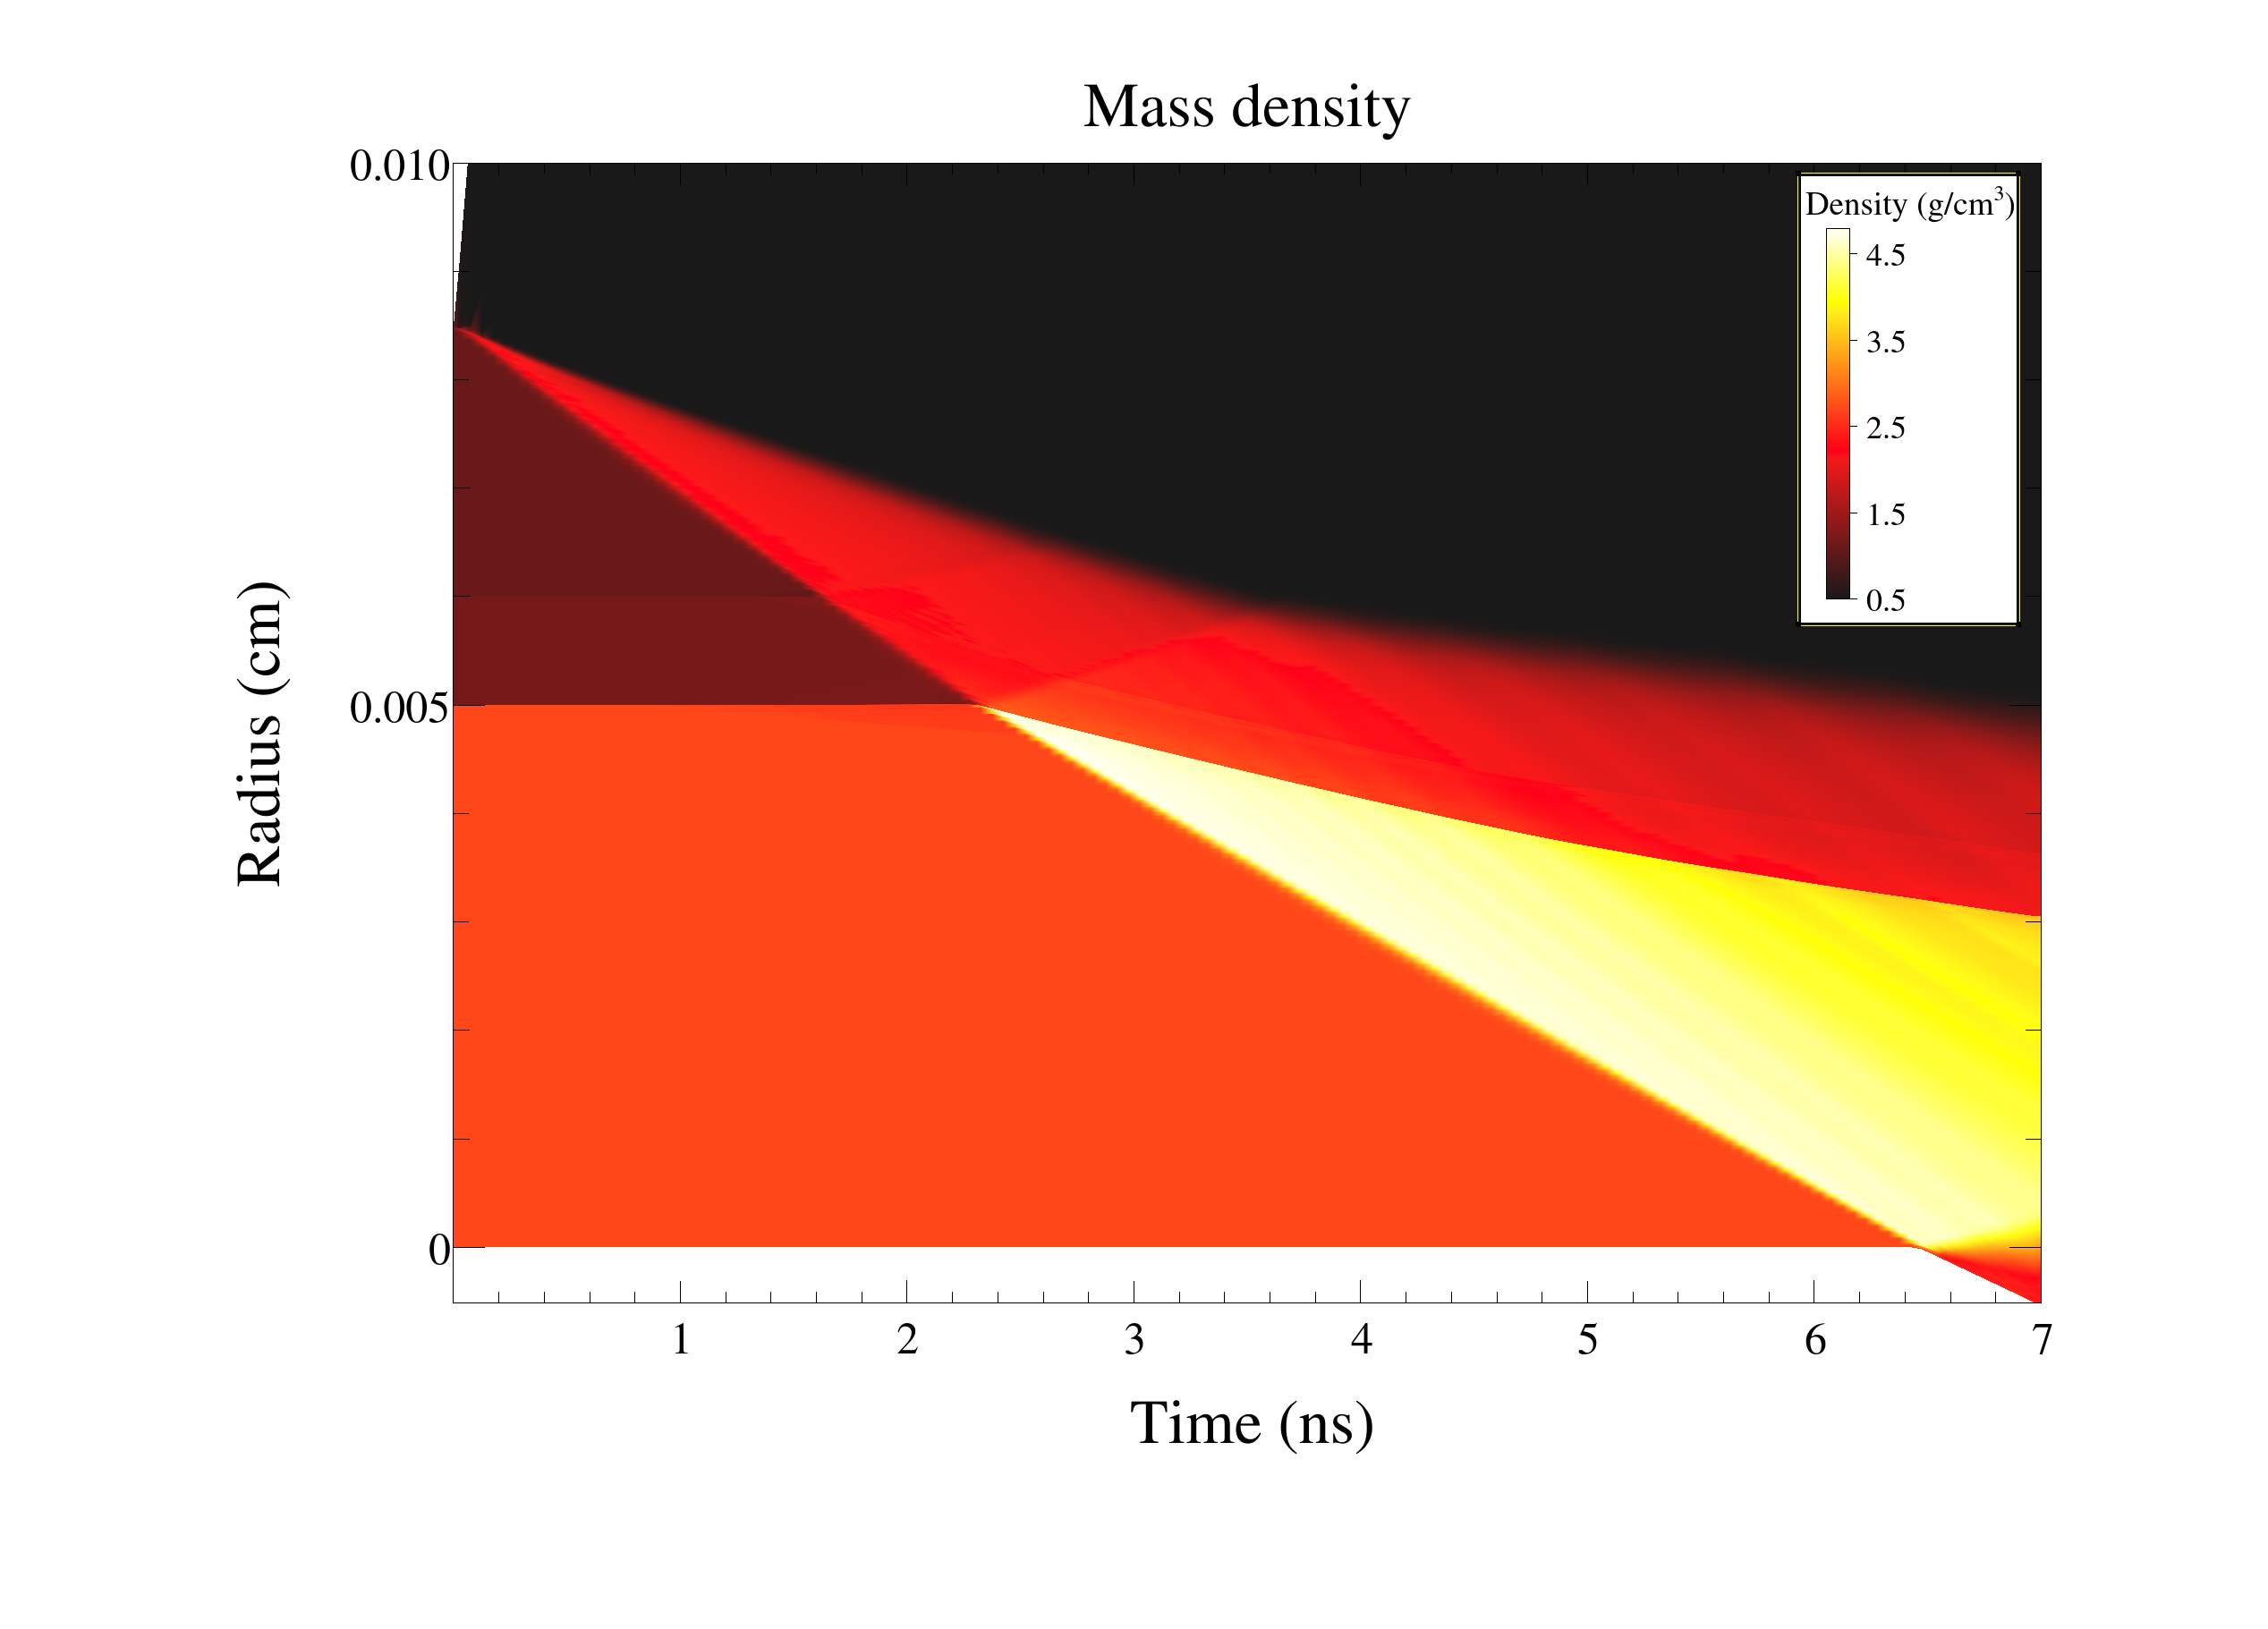}
\put(4,60){\large\bfseries (a)}
\end{overpic}
\hfill
\begin{overpic}[width=0.49\linewidth,trim=190 140 120 120,clip]{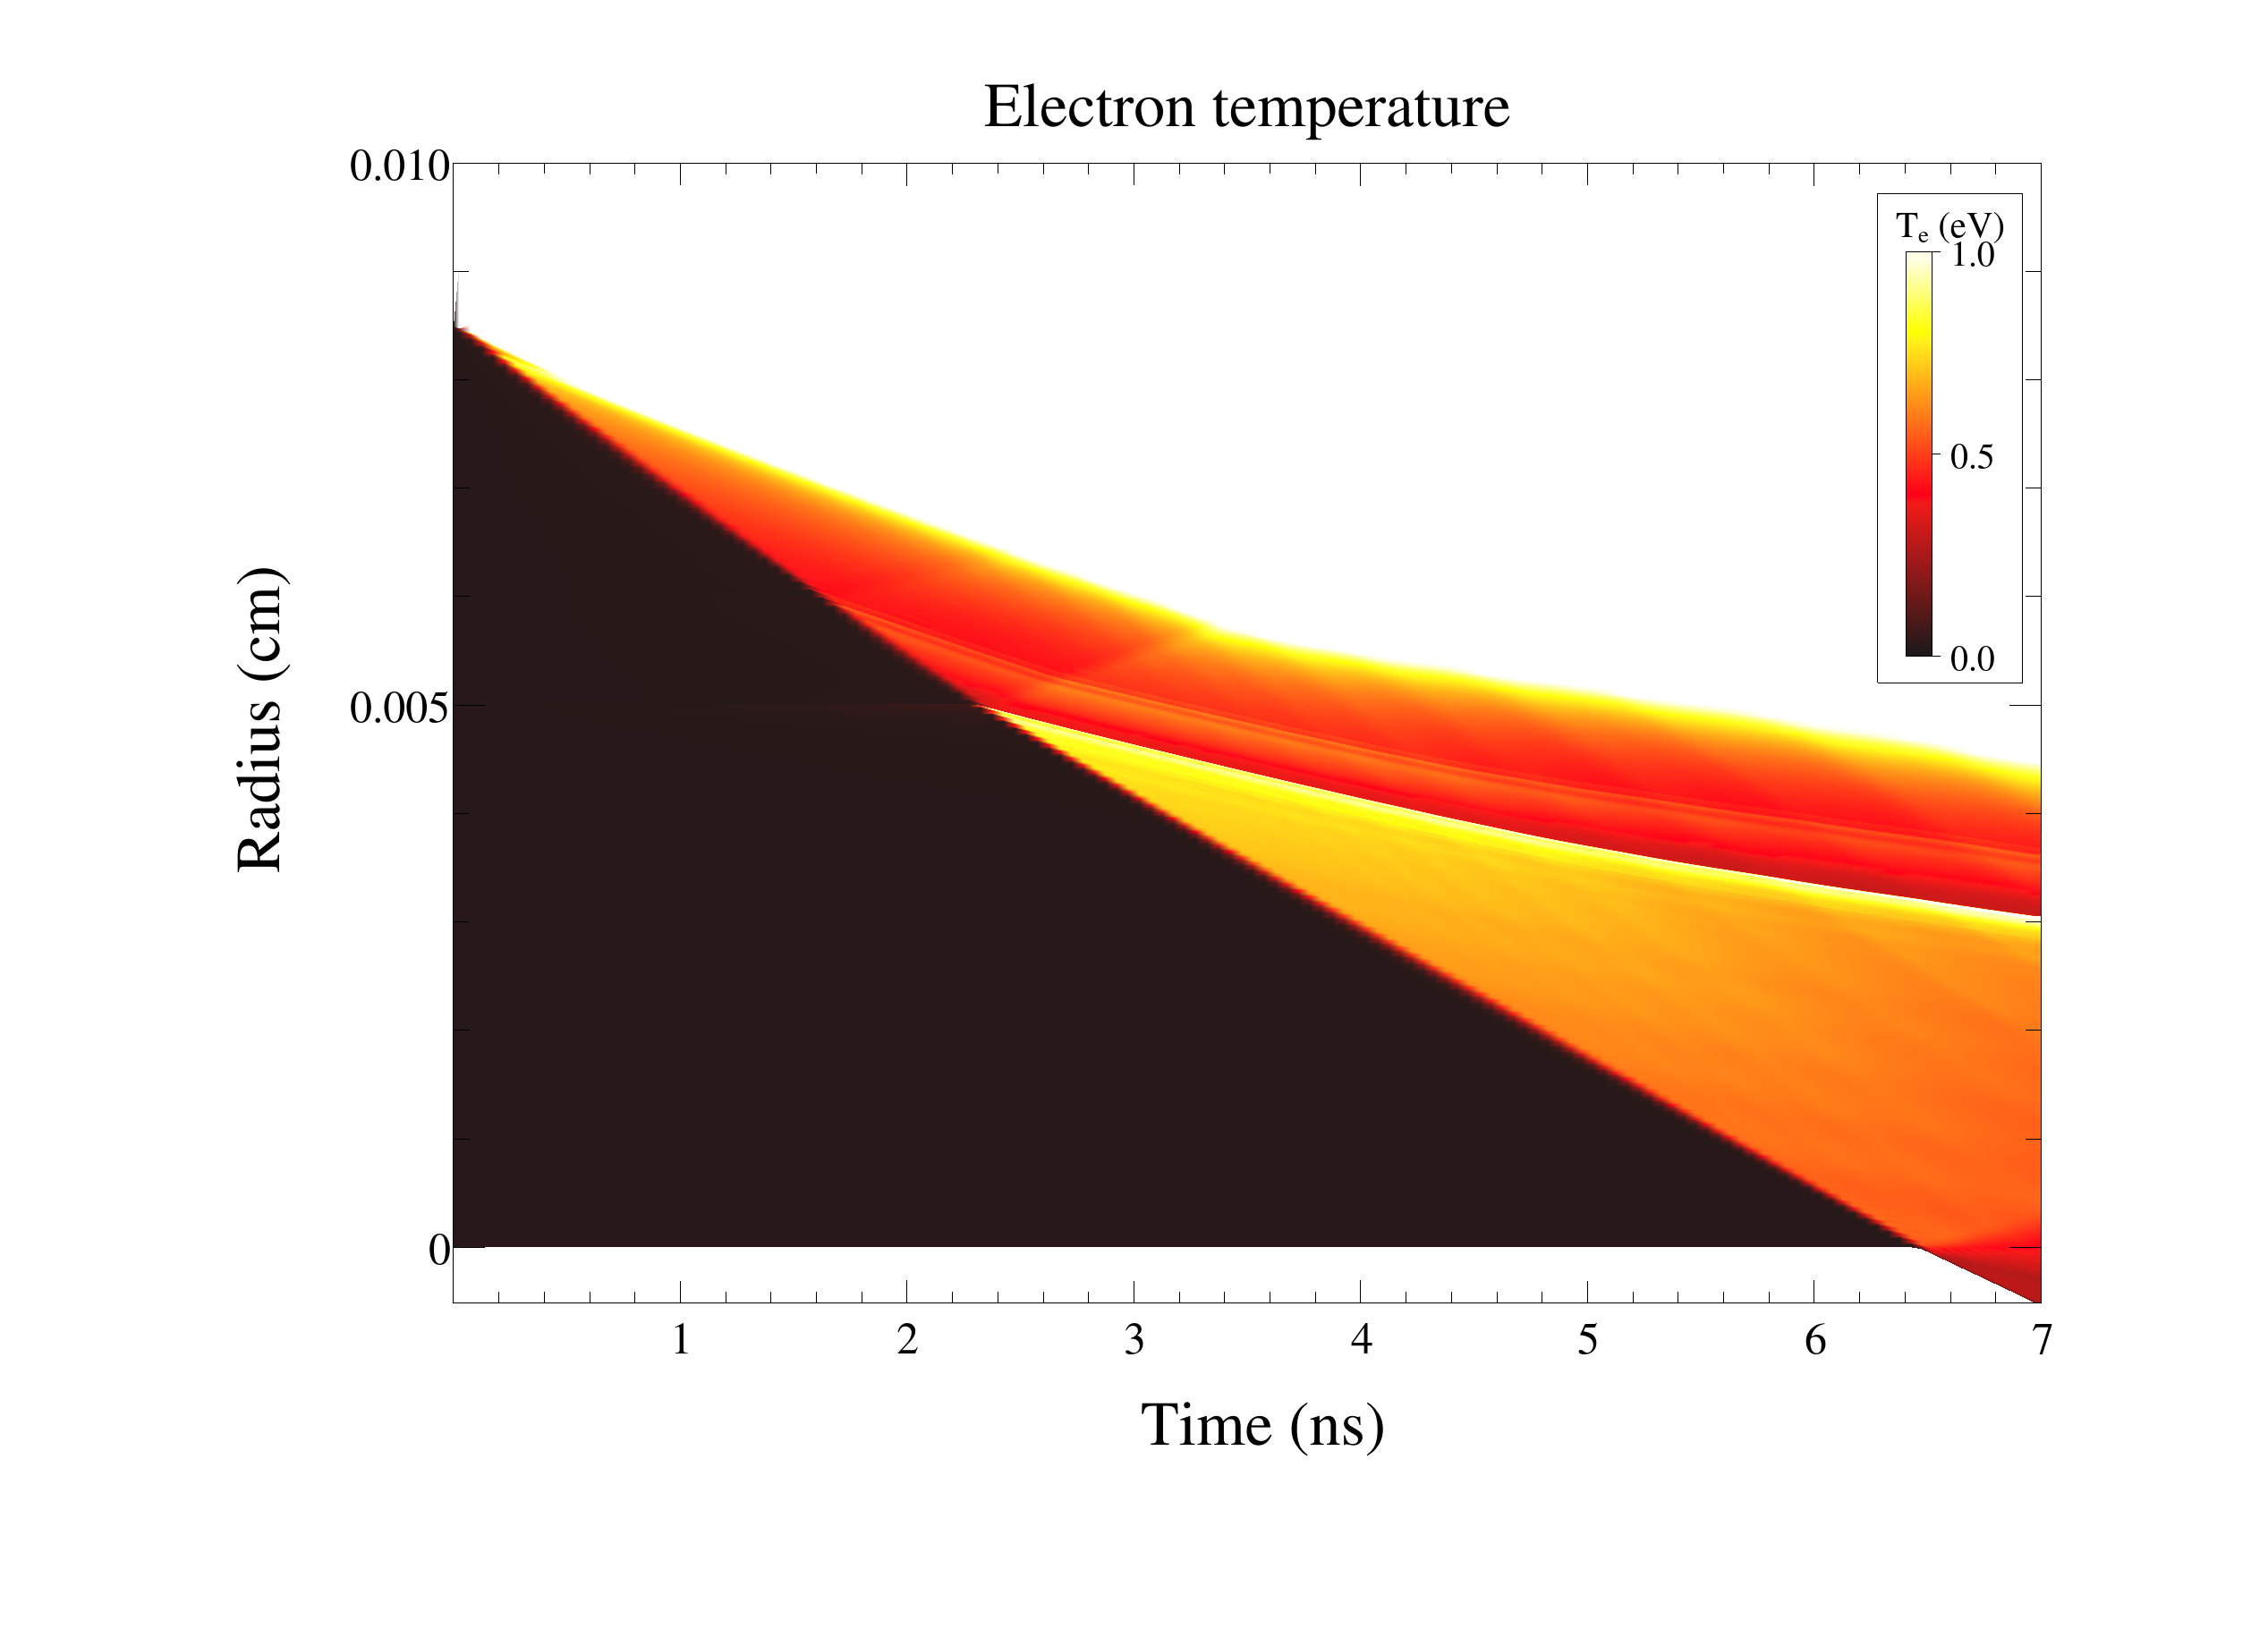}
\put(4,60){\large\bfseries (b)}
\end{overpic}

\caption{\textbf{Hydrodynamic space–time maps from HELIOS-CR.}
\textbf{(a)} Mass density $\rho(r,t)$ and \textbf{(b)} electron temperature $T_e(r,t)$ from the calibrated HELIOS-CR simulation of the full target stack. The maps illustrate the formation of the compressed aluminium layer prior to breakout and the weak temperature gradient across the region probed by XRTS and XRD near the XFEL probe time $t_\mathrm{pp}=6.3$ ns.}

\label{fig:hydro_2d}

\end{figure*}

\textbf{DiPOLE shot-to-shot stability.}
Figure~\ref{fig:dipoole_stability} summarizes the recorded pulse energies during XRTS acquisition. Nearly all shots lie within $\pm0.75\%$ of the 26~J median (standard deviation $<1\%$), consistent with the stable drive conditions assumed in the HELIOS-CR modeling.

\begin{figure}[t]
  \centering
  \includegraphics[width=0.50\linewidth]{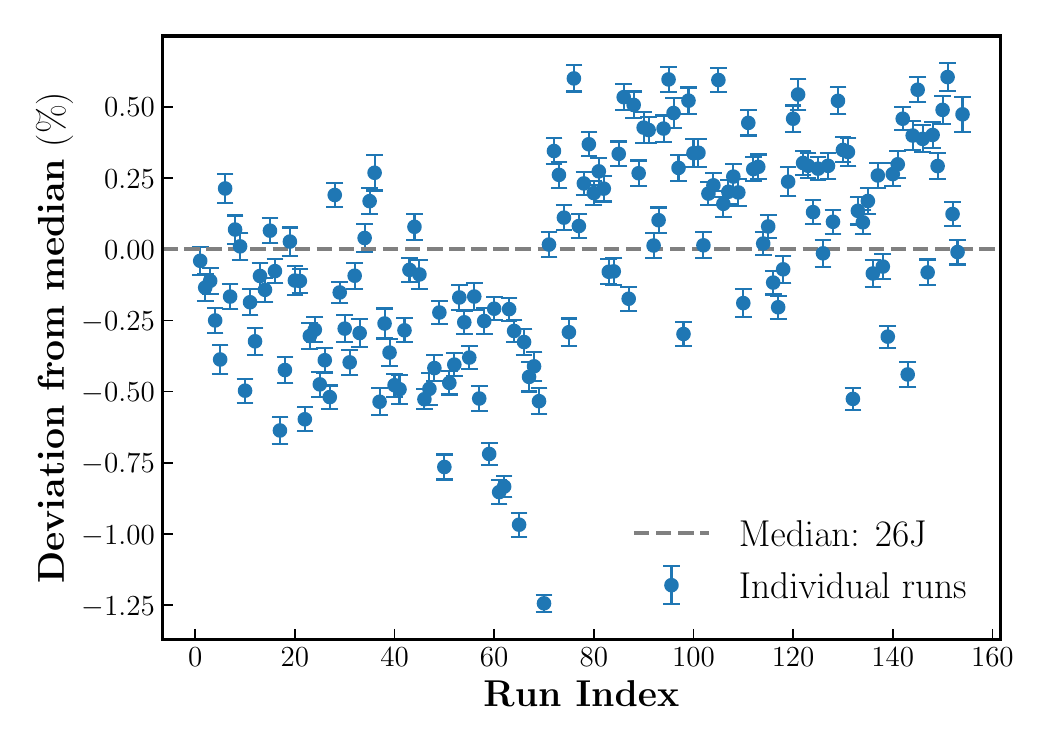}
  \caption{\textbf{Shot-to-shot variation of the DiPOLE drive.}
  Pulse energies recorded immediately prior to XFEL shots. The solid line marks the median energy (26~J); the shaded band denotes the $\pm0.75\%$ interval. Stable drive conditions enable reproducible compression and quantitative spectral averaging.}
  \label{fig:dipoole_stability}
\end{figure}

\SMsection{Source-and-instrument function (SIF) and spectral model}{sec:S2}

All experiment-theory comparisons use a measured source-and-instrument function (SIF) determined independently for each scattering geometry from cold (ambient) aluminium targets acquired under identical spectrometer settings as the driven shots. The representative SIF used in the main validation package is shown in the End Matter (the SIF figure). The need for a per-geometry SIF arises from small but measurable geometry-dependent changes in the effective focusing conditions of the von H\'amos spectrometer.

For each scattering vector, the quasi-elastic line from cold aluminium was fitted by the sum of two Voigt profiles: a narrow seeded component (FWHM $\approx3.3$~eV) and a weak pedestal (FWHM $\approx22.7$~eV, relative peak height $\approx0.08$). The resulting effective resolution is $3.5$~eV (FWHM). These geometry-specific SIFs are held fixed for all driven-shot fits and are used in all convolutions of theoretical spectra.

For quantitative analysis, spectra are normalised to the elastic line and fitted with the same minimal model used in the main text. The elastic component is fixed by the measured SIF. The plasmon contribution is represented by a Voigt profile whose Gaussian width is fixed by the SIF and whose Lorentzian width is a free non-negative parameter; detailed balance is enforced between the energy-gain and energy-loss sides through the factor $\exp(-\omega/k_B T_e)$. A low-order polynomial background accounts for weak continuum and residual ablator contributions bounded in Sec.~\ref{sec:S6}.

For theoretical spectra, the dynamic structure factor is convolved with the geometry-specific SIF and combined with an elastic contribution,
\begin{equation}
  I_{\mathrm{model}}(k,\omega)
  = I_{\mathrm{el}}\,\mathrm{SIF}_{k}(\omega)
    + I_{\mathrm{inel}}\!\left[S(k,\omega) * \mathrm{SIF}_{k}(\omega)\right],
\end{equation}
where $\mathrm{SIF}_{k}(\omega)$ denotes the source-and-instrument function measured for the corresponding scattering geometry and $I_{\mathrm{el}}/I_{\mathrm{inel}}$ is the fitted elastic-to-inelastic intensity ratio. Both the spectral fits and all theoretical curves therefore use the same geometry-specific SIF, ensuring that differences between experiment and theory arise from the underlying $S(k,\omega)$ rather than from instrumental broadening.

\SMsection{TDDFT and DFT-MD settings and convergence}{sec:S3}

%\textcolor{blue}{
To model the XRD data, one requires the static ion--ion structure factor, $S_{ii}(k)$, which we computed using KSDFT-based molecular dynamics of ions. In these simulations, the electrons are treated within conventional DFT and are assumed to respond instantaneously to changes in nuclear positions (Born--Oppenheimer approximation).
Modelling the XRTS spectrum requires access to the dynamic electron--electron structure factor, $S_{ee}(k,\omega)$. This quantity cannot be obtained from standard DFT-MD simulations and instead requires a time-dependent treatment of the electronic response. For that, we used linear response TD-DFT.
%}
\paragraph{KSDFT framework.}
The Kohn--Sham density functional theory (KSDFT) calculations were performed with the open-source \textsc{Quantum~ESPRESSO} suite~\cite{Giannozzi_2017,Giannozzi_jcp_2020,PP_ESPRESSO_2022}, using norm-conserving pseudopotentials and the PBE exchange-correlation functional. Electronic occupations were treated at finite temperature consistent with the target electron temperature, and all plane-wave calculations used a kinetic-energy cut-off of 50~Ry, which was verified to yield converged total energies and structural properties for warm dense Al in the considered density range.

\paragraph{TDDFT.}
Dynamic structure factors $S(k,\omega)$ were computed using the Liouville--Lanczos linear-response implementation of time-dependent density functional theory (TDDFT) as implemented in \textsc{turboTDDFT}~\cite{TIMROV2015460,Carnimeo_JCTC_2023}. All calculations employed the PBE exchange-correlation functional with its adiabatic generalised-gradient (AGGA) kernel and the norm-conserving pseudopotential \texttt{Al.pbe-rrkj.UPF}. Each simulation cell contained 32~Al ions in a periodic cubic box, sampled on a $10\times10\times10$ electronic $k$-mesh with a plane-wave cut-off energy of 50~Ry. Lorentzian broadenings $\eta=\{0.1,0.1,0.3,0.5\}$~eV were used for the four momentum transfers $k = \{0.99,1.28,1.57,2.57\}~\si{\per\angstrom}$; these parameters correspond to the intrinsic frequency-space smearing in the Liouville--Lanczos algorithm and are small compared with the experimental SIF width, so that the dominant broadening in experiment--theory comparisons is set by the measured 3.5~eV (FWHM) resolution. Spectra were converged with $\sim10^{5}$ Lanczos coefficients obtained from over $5\times10^{3}$ iterations and averaged over ten independent ionic configurations extracted from the DFT-MD trajectory. Frozen-ion snapshots are appropriate because the probe duration (25~fs) is far shorter than ionic timescales. Electron densities and temperatures used as input were taken directly from the HELIOS-CR profiles discussed in End Matter, Experimental state determination, using the same set of $N=4$ densities spanning $3.75$--$4.5~\mathrm{g\,cm^{-3}}$ at $T\approx0.6$~eV that enter the density averaging of Eq.~(S1).

\paragraph{DFT-MD.}
The ionic structure factor $S_{ii}(k)$ was determined from finite-temperature DFT molecular dynamics, also performed with \textsc{Quantum~ESPRESSO}. Simulations used a 108-atom cubic supercell with periodic boundary conditions, a $2\times2\times2$ electronic $k$-mesh, and a plane-wave cut-off of 50~Ry. A Nos\'e--Hoover thermostat maintained the target temperature, and ionic trajectories were propagated with a 1~fs time step. After equilibration, $8\times10^{3}$ configurations were sampled to generate ensemble-averaged pair correlation functions and $S_{ii}(k)$. Finite-size effects were assessed by comparing results from 32-atom and 108-atom cells; both yielded indistinguishable $g(r)$ and $S_{ii}(k)$ over the reported $k$-range, confirming convergence. DFT-MD simulations were performed at the same set of densities and temperature as the TDDFT calculations, matching the HELIOS-CR density and temperature window. Further methodological details follow Refs.~\cite{TIMROV2015460,Carnimeo_JCTC_2023,ullrich2012time}.

\SMsection{Full XRTS data set and model comparison}{sec:S4}

Figure~\ref{fig:fullset} shows the full driven data set together with density-averaged, SIF-convolved TDDFT, static-LFC, and RPA spectra. TDDFT reproduces the measured peak positions and line shapes across the full momentum range, whereas UEG-based RPA and static-LFC models remain too narrow and too weakly damped. At $k = 2.57~\si{\per\angstrom}$ the mode is strongly Landau damped and only $E_{\mathrm{peak}}(k)$ is used quantitatively~\cite{Fortmann_PRE_2010,Dornheim_PRL_2020_ESA,preston2019momentum}.

\begin{figure*}[t]
  \centering
  \includegraphics[width=0.40\linewidth]{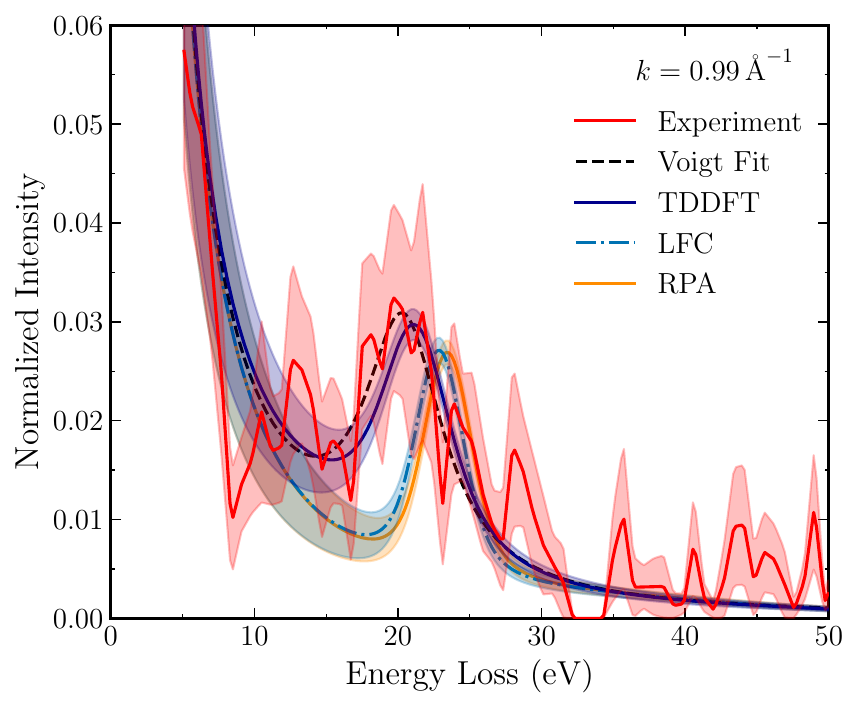}
  \includegraphics[width=0.40\linewidth]{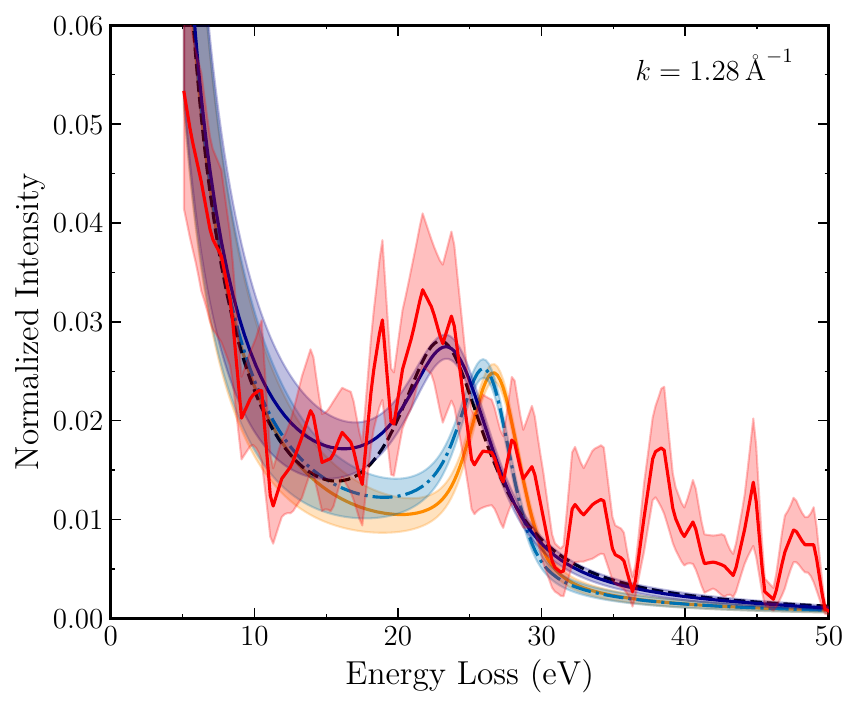}\\
  \includegraphics[width=0.40\linewidth]{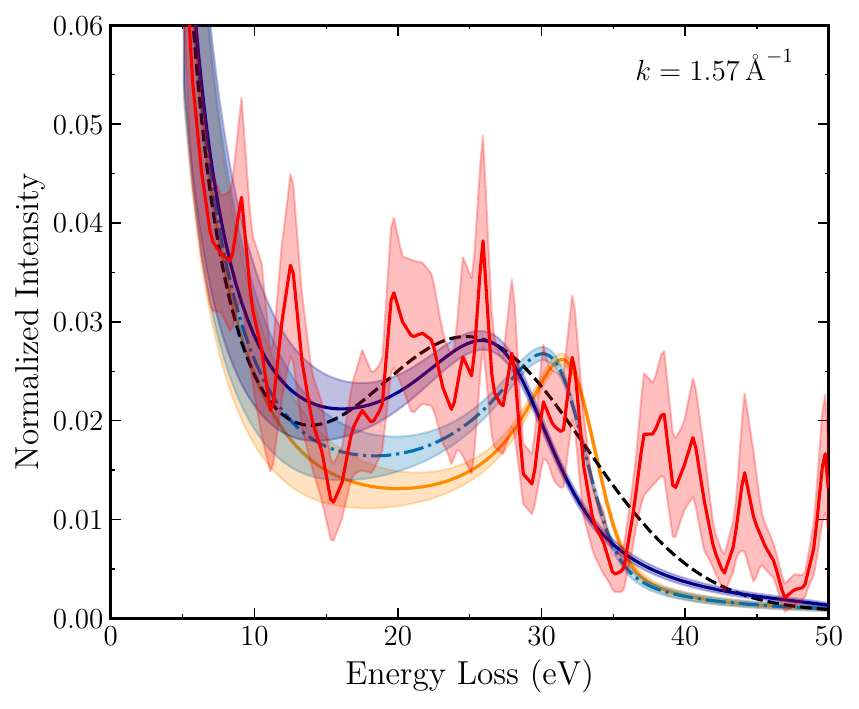}
  \includegraphics[width=0.40\linewidth]{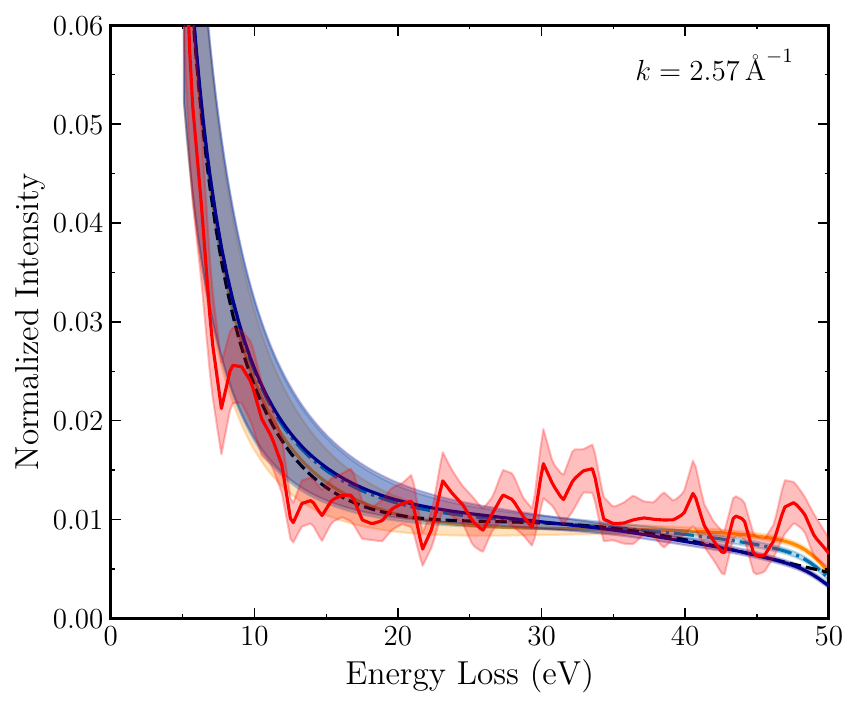}
  \caption{\textbf{Full comparison set.}
  Driven spectra (red, $1\sigma$ bands) with TDDFT (blue), static-LFC (cyan), and RPA (gold), all evaluated over the HELIOS-CR/XRD density window, density-averaged, and SIF-convolved. Dashed black curves show the fitted Voigt components used to extract $E_{\mathrm{peak}}(k)$.}
  \label{fig:fullset}
\end{figure*}

\SMsection{Uncertainty Quantification}{sec:S5}

The error bars in the main-text plasmon-dispersion figure combine the fit covariance from SIF-constrained Voigt fits, the absolute energy calibration, angle-to-$k$ conversion, state averaging over the HELIOS-CR/XRD density window, and the spread associated with the independently fitted SIFs. During the experiment no measurable drift of the incident x-ray energy was observed on the scale relevant for the reported plasmon positions, and the SIF fits were constrained so that the elastic peak remained centred at zero energy transfer. The contribution from absolute energy drift to the quoted $E_{\mathrm{peak}}(k)$ uncertainties is therefore negligible compared with the other terms retained below.

For the angle-to-$k$ conversion, $k=(4\pi/\lambda)\sin(\theta/2)$, differentiation yields
\begin{equation}
  \delta k = \frac{2\pi}{\lambda}\cos(\theta/2)\,\delta\theta,
\end{equation}
and we adopt a conservative $\delta\theta=\pm0.5^\circ$ that includes mechanical and encoder precision, HAPG mosaicity ($\sim0.1^\circ$), and the small elastic--inelastic centroid offset.

State uncertainties are propagated by evaluating each model over the HELIOS-CR/XRD density window defined in Sec.~\ref{sec:S1} at fixed temperature $T \approx 0.6~\si{\electronvolt}$ and density-averaging the spectra before SIF convolution. In addition, the spread between the independently fitted SIF profiles at different scattering angles (Sec.~\ref{sec:S2}; End Matter, Instrumental response and spectral analysis) is used to estimate the impact of response-function uncertainty on extracted peak positions. The above contributions are combined in quadrature to obtain the error bars on $E_{\mathrm{peak}}(k)$ and, where resolvable, on the reported widths. When the width is not resolvable because of overlap with the particle-hole continuum at large $k$, only $E_{\mathrm{peak}}(k)$ is quoted.

\SMsection{Ablator response and ray-tracing validation}{sec:S6}

Ambient ablator-only spectra bound the Kapton contribution to the high-loss wing. Across the range of ablator scalings consistent with the ambient data, subtraction reduces the $>30$~eV tail without shifting the plasmon peak by more than the quoted experimental error bars (Fig.~\ref{fig:ablator}). In experiment-theory comparisons, the elastic-to-inelastic ratio is fitted, so ablator elastic scattering is absorbed into that parameter and does not bias $E_{\mathrm{peak}}(k)$.

To verify instrumental contributions, we ray-trace the HAPG(004) von H\'amos spectrometer (80~mm$\times$30~mm, 40~$\mu$m thick, 120~mm radius) using HEART~\cite{HEART}, with wrapped-Lorentzian mosaicity $0.07^\circ$ and a Voigt intrinsic rocking curve (Gaussian 25.35~$\mu$rad, Lorentzian 5.00~$\mu$rad). The measured seed-plus-pedestal source spectrum and density-averaged TDDFT $S(k,\omega)$ serve as inputs. Simulations with $10^{9}$ photons reproduce the elastic line shape and confirm that both the negative-loss tail and the high-loss decay follow the SIF, not additional plasma emission~\cite{Zastrau2021,siegfried_review,GawneMosaic}.

\begin{figure*}[ht]
  \centering
  \includegraphics[width=0.75\linewidth]{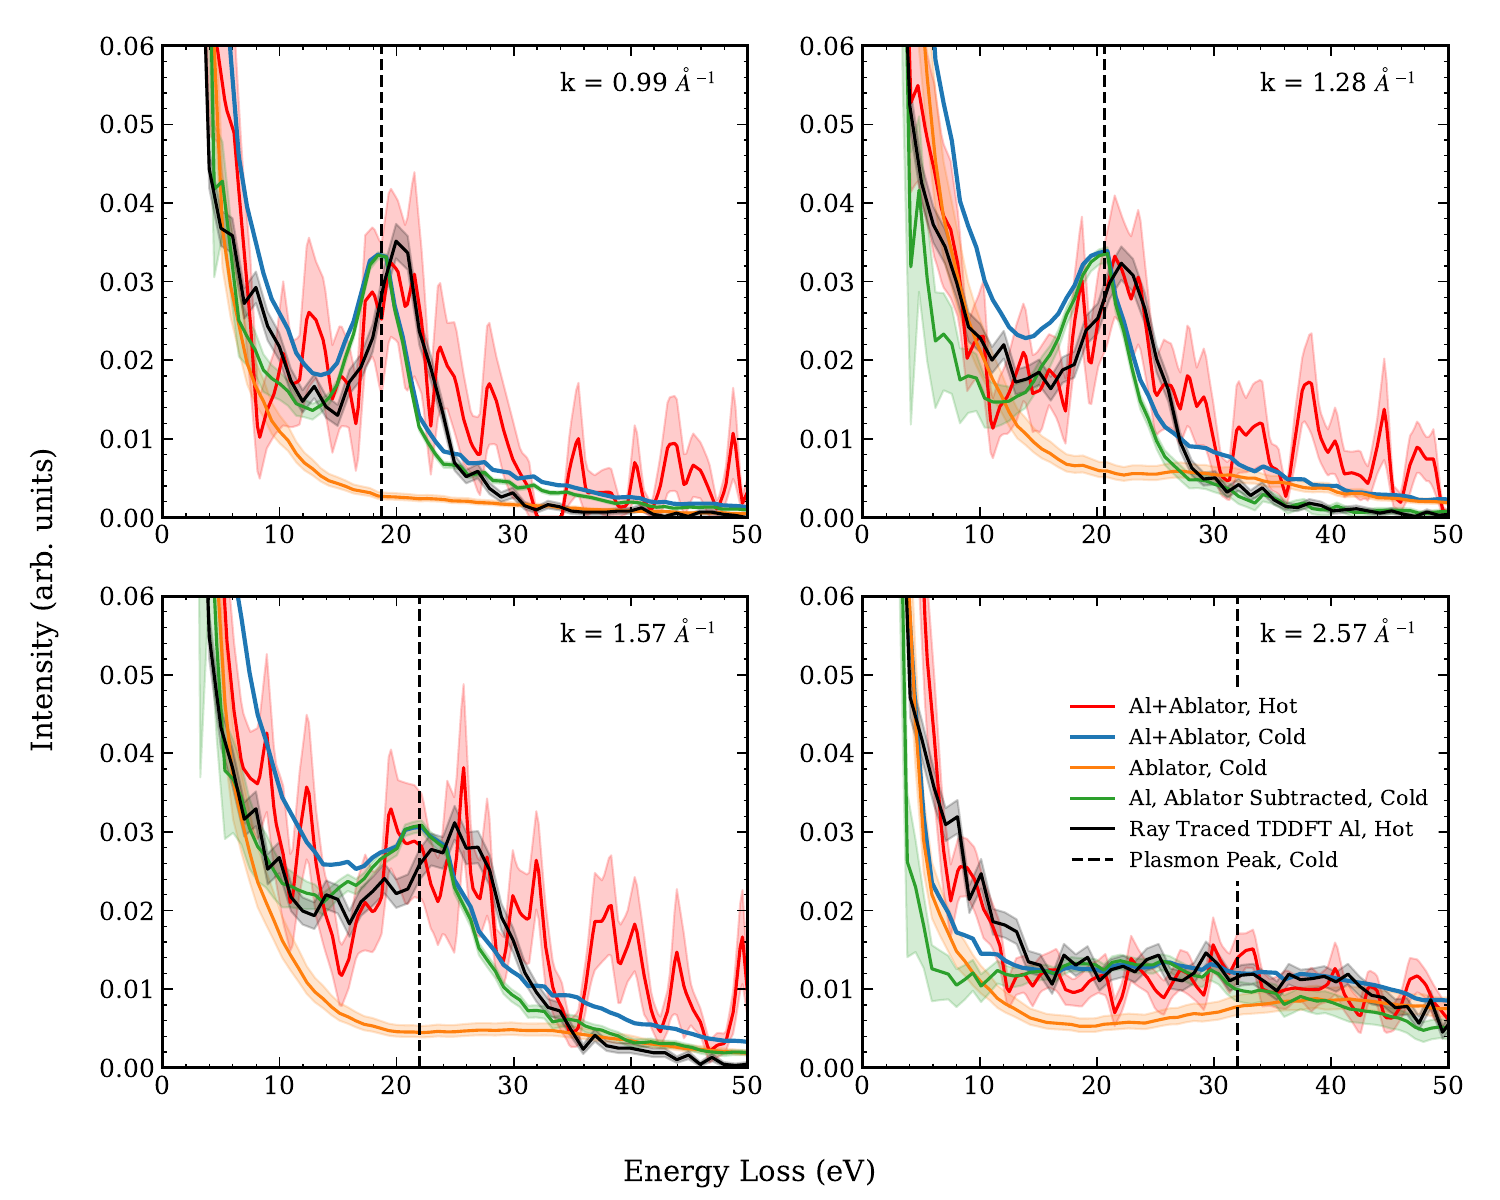}
  \caption{\textbf{Ablator response and ray-tracing validation.}
  Ambient full target (blue), ablator-only (orange), and an ``Al-only'' estimate (green) after ablator subtraction with bounds. Driven spectra (red) and ray-traced TDDFT (black) show that the $>30$~eV wing is ablator-dominated and that the measured tails are consistent with the SIF response.}
  \label{fig:ablator}
\end{figure*}

\SMsection{Ambient validation and calibration cross-checks}{sec:S7}

Ambient plasmon peak positions measured with the same geometry agree with recent European XFEL reference data at low $k$ and soften towards the pair continuum at large $k$ (Fig.~\ref{fig:ambient}), consistent with Ref.~\cite{Gawne2024xray}. Over the common $k$ range, the present and reference dispersions agree within the combined experimental uncertainties, validating the absolute energy scale and the scattering angles used in the Letter.

\begin{figure}[t]
  \centering
  \includegraphics[width=0.50\linewidth]{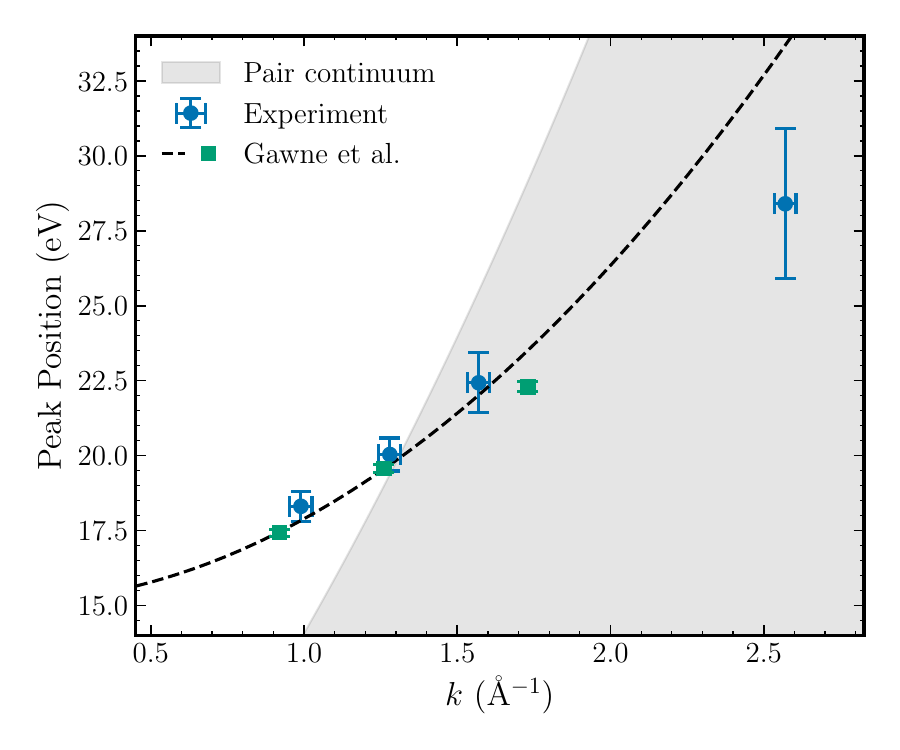}
  \caption{\textbf{Ambient cross-check.}
  Present ambient Al dispersion (blue) compared with ambient reference data (green). Dashed curve: quadratic Bohm--Gross fit. Shaded region: onset of the particle-hole continuum.}
  \label{fig:ambient}
\end{figure}

\SMsection{Raw XRD examples}{sec:S8}

Representative ambient and driven XRD spectra used for $S_{ii}(k)$ extraction are shown in Fig.~\ref{fig:XRD}. The ambient Bragg peak is masked during the liquid-state analysis, and only the diffuse driven signal is used for comparison with DFT-MD $S_{ii}(k)$ in the HELIOS-CR density window.

\begin{figure*}[ht]
  \centering
  \includegraphics[width=0.4\linewidth]{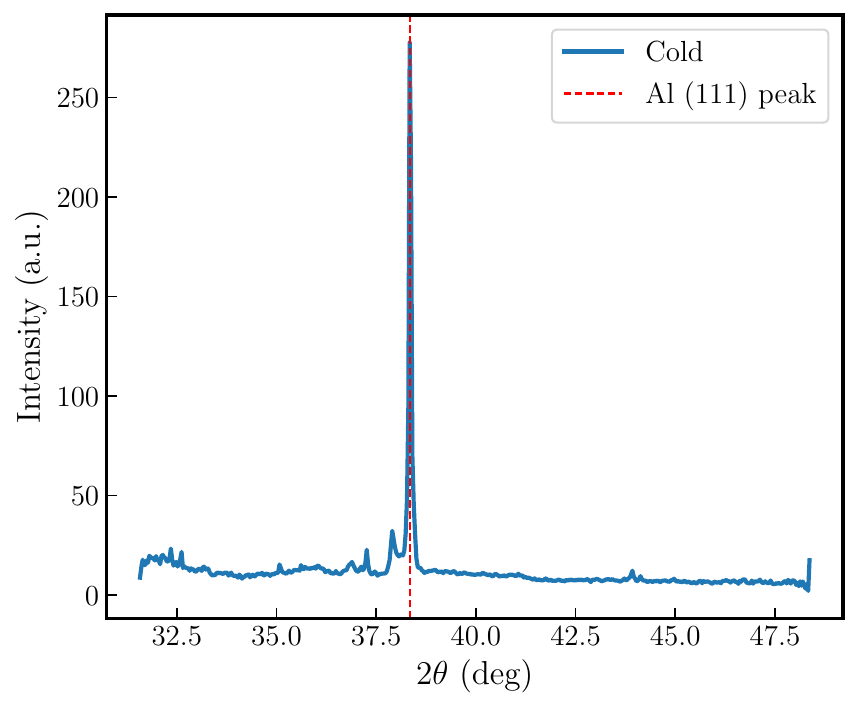}
  \includegraphics[width=0.4\linewidth]{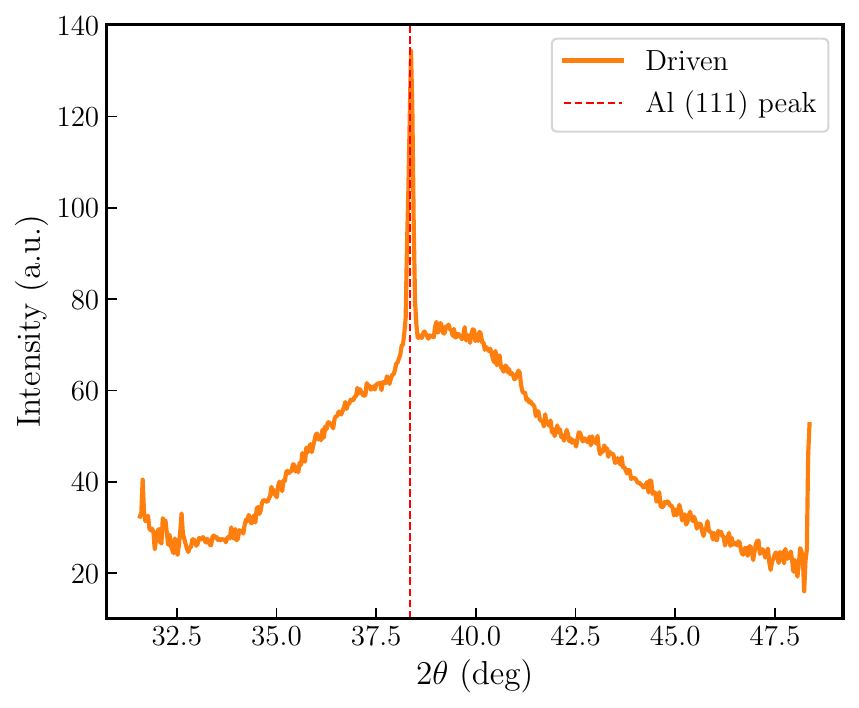}
  \caption{\textbf{Raw XRD examples.}
  Left: ambient Al with a sharp (111) peak. Right: driven liquid-like diffuse scattering; the residual ambient peak originates from unshocked regions and is excluded from the $S_{ii}(k)$ analysis.}
  \label{fig:XRD}
\end{figure*}

\bibliographystyle{apsrev4-2}
\bibliography{references_PRL}

\end{document}
